# Supplementary material for: Do Audio-Language Models Understand Linguistic Variations?
Source: arXiv:2410.16505 source file (2025-02-20)
Supplement: Supplementary file 1 [file additional_results_best.tex]

\begin{table*}[!ht]
\resizebox{\textwidth}{!}{
\begin{tabular}{@{}cccccccccc@{}}
\toprule
\multicolumn{2}{c}{\textbf{Retrieval Type $\longrightarrow$}}           & \multicolumn{4}{c}{\textbf{Text-to-Audio Retrieval}}                 & \multicolumn{4}{c}{\textbf{Audio-to-Text Retrieval}}                 \\ \midrule
\multirow{2}{*}{\textbf{Benchmark}}   & \multirow{2}{*}{\textbf{Model}}  & \multicolumn{2}{c}{R@1 $\uparrow$} & \multicolumn{2}{c}{R@10 $\uparrow$} & \multicolumn{2}{c}{R@1 $\uparrow$} & \multicolumn{2}{c}{R@10 $\uparrow$}  \\ \cmidrule(l){3-10} 
                             &                        & TEST & TEST-P & TEST & TEST-P & TEST & TEST-P & TEST & TEST-P   \\ \midrule
\multirow{2}{*}{AudioCaps}   & CLAP                   & \textbf{07.02}           & 04.62            & 48.71         & 35.72           & \textbf{08.78}           & 05.35            & \textbf{49.15}         & 29.72           \\
                             & RobustCLAP             & 06.50          & \textbf{05.89}            & \textbf{49.49}         & \textbf{46.94}           & 07.48           & \textbf{07.71}            & 46.56         & \textbf{43.80}            \\ \midrule
\multirow{2}{*}{Clotho}      & CLAP                   & 38.08          & 30.90            & 81.24         & 75.88           & 37.03          & 30.72           & 81.91         & 74.83           \\
                             & RobustCLAP             & \textbf{38.27}         & \textbf{37.12}           & \textbf{81.53}         & \textbf{80.76}           & \textbf{39.43}         & \textbf{37.32}           & \textbf{82.49}         & \textbf{82.30}           \\ \midrule
\multirow{2}{*}{Audioset SL} & CLAP                   & 12.78          & 11.83           & 48.20          & 42.76           & \textbf{16.52}          & 11.90            & \textbf{52.75}         & 43.71           \\
                             & RobustCLAP             & \textbf{15.77}         & \textbf{14.89}           & \textbf{49.83}         & \textbf{47.52}           & 15.84         & \textbf{14.41}           & 50.37         & \textbf{47.99 }          \\ \midrule
\multirow{2}{*}{SoundDesc}   & CLAP                   & 04.95           & 03.66            & 21.91         & 16.95           & 03.23           & 02.34            & 17.75         & 13.63           \\
                             & RobustCLAP             & \textbf{05.45}          & \textbf{04.12}            & \textbf{23.05}         & \textbf{20.83}          & \textbf{03.78}          & \textbf{02.95}            & \textbf{19.08}         & \textbf{16.92}           \\ \midrule
\multirow{2}{*}{DCASE}       & CLAP                   & 15.05          & 11.84           & 49.25         & 42.63           & 17.25          & 10.93           & \textbf{54.86}         & 43.53           \\
                             & RobustCLAP             & \textbf{16.75}         & \textbf{14.54}           & \textbf{54.26}         & \textbf{49.75}           & \textbf{14.84}         & \textbf{13.14}           & 48.65         & \textbf{45.94}           \\ \bottomrule
\end{tabular}}
\caption{\small T-A and A-T retrieval results for CLAP and RobustCLAP across the original test set (TEST) and the paraphrased test sets (TEST-P). We observe for this new variant of CLAP (630k-fusion-best) again across the benchmark there is a consistent and considerable drop in retrieval performance. When we derive RobustCLAP from this CLAP variant, we again notice the trend where there is improvement in general retrieval recall on \textbf{TEST} and mitigation of the drop in score in TEST-P. The best scores for each benchmark are highlighted in \textbf{bold}. This CLAP variant can be found here: \url{https://huggingface.co/lukewys/laion_clap/blob/main/630k-fusion-best.pt}}
\label{tab:main_result_additional}
\end{table*}
